# Supplementary material for: Nonlinear corrections in the quantization of a weakly nonideal Bose gas at zero temperature. II. The general case
Source: arXiv:2206.06316 ancillary file (2023-01-03)
Supplement: Supplementary file 1 [file commutators_coeff_general.pdf]

```

→ /* Definitions (130)-(133) */
/* \gamma_{j}/\omega=J, \gamma_{l}/\omega=L, \gamma_{j+l}/\omega=S */
/* \tilde v_{j}=vj, \tilde v_{l}=vl, \tilde v_{j+l}=vs */;

(%i1) /* M_{j,l}^{\star}d_{l}\omega/c_{j}=Mp1(J,L,S,vj,vl,vs) */

Mp1(J,L,S,vj,vl,vs):=(1/(2*vj*L*((J+L)^2-S^2)))*((J+L+sqrt(S^2+vs^2))
    *(vl*(vj+vs)*(J-sqrt(J^2+vj^2))+vj*(vl+vs)*(L-sqrt(L^2+vl^2))+vj*vl*(vj+vl))
    -vs*(vj+vl)*(J-sqrt(J^2+vj^2))*(L-sqrt(L^2+vl^2))
    -vl*vs*(vl+vs)*(J-sqrt(J^2+vj^2))-vj*vs*(vj+vs)*(L-sqrt(L^2+vl^2)));

(%o1) Mp1(J,L,S,vj,vl,vs):=

$$\frac{1}{2 v j L \left( (J+L)^2 - S^2 \right)} \left( (J+L + \sqrt{S^2 + v s^2}) \right. \\
\left. \left( v l (v j + v s) (J - \sqrt{J^2 + v j^2}) + v j (v l + v s) (L - \sqrt{L^2 + v l^2}) + v j v l (v j + v l) \right) - v s (v j + v l) (J - \sqrt{J^2 + v j^2}) \right. \\
\left. (L - \sqrt{L^2 + v l^2}) + (-v l) v s (v l + v s) (J - \sqrt{J^2 + v j^2}) + (-v j) v s (v j + v s) (L - \sqrt{L^2 + v l^2}) \right)$$


(%i2) /* M_{j,-j-l}^{\star}d_{j+l}\omega/c_{j}=Mp2(J,L,S,vj,vl,vs) */

Mp2(J,L,S,vj,vl,vs):=(1/(2*vj*S*((J+S)^2-L^2)))*((J+S+sqrt(L^2+vl^2))
    *(vs*(vj+vl)*(J-sqrt(J^2+vj^2))+vj*(vl+vs)*(S-sqrt(S^2+vs^2))+vj*vs*(vj+vs))
    -vl*(vj+vs)*(J-sqrt(J^2+vj^2))*(S-sqrt(S^2+vs^2))
    -vl*vs*(vl+vs)*(J-sqrt(J^2+vj^2))-vj*vl*(vj+vl)*(S-sqrt(S^2+vs^2)));

(%o2) Mp2(J,L,S,vj,vl,vs):=

$$\frac{1}{2 v j S \left( (J+S)^2 - L^2 \right)} \left( (J+S + \sqrt{L^2 + v l^2}) \right. \\
\left. \left( v s (v j + v l) (J - \sqrt{J^2 + v j^2}) + v j (v l + v s) (S - \sqrt{S^2 + v s^2}) + v j v s (v j + v s) \right) - v l (v j + v s) (J - \sqrt{J^2 + v j^2}) \right. \\
\left. (S - \sqrt{S^2 + v s^2}) + (-v l) v s (v l + v s) (J - \sqrt{J^2 + v j^2}) + (-v j) v l (v j + v l) (S - \sqrt{S^2 + v s^2}) \right)$$


```

(%i3) /\*  $M_{\{j,-1\}}^{\{\star\}} c_{\{1\}} \omega / c_{\{j\}} = Mm1(J,L,S,vj,vl,vs)$  \*/

$Mm1(J,L,S,vj,vl,vs) := (1/(2 \cdot vj \cdot L \cdot ((J-L)^2 - S^2))) \cdot ((J-L + \sqrt{S^2 + vs^2}) \cdot (vl \cdot (vj+vs) \cdot (\sqrt{J^2 + vj^2} - J) + vj \cdot (vl+vs) \cdot (\sqrt{L^2 + vl^2} + L) - vj \cdot vl \cdot (vj+vl)) + vs \cdot (vj+vl) \cdot (\sqrt{J^2 + vj^2} - J) \cdot (\sqrt{L^2 + vl^2} + L) - vl \cdot vs \cdot (vl+vs) \cdot (\sqrt{J^2 + vj^2} - J) - vj \cdot vs \cdot (vj+vs) \cdot (\sqrt{L^2 + vl^2} + L));$

(%o3)  $Mm1(J,L,S,vj,vl,vs) := \frac{1}{2 vj L \left( (J-L)^2 - S^2 \right)} \left( (J-L + \sqrt{S^2 + vs^2}) \left( vl (vj+vs) (\sqrt{J^2 + vj^2} - J) + vj (vl+vs) (\sqrt{L^2 + vl^2} + L) + (-vj) vl (vj+vl) \right) + vs (vj+vl) \right. \\ \left. (\sqrt{J^2 + vj^2} - J) (\sqrt{L^2 + vl^2} + L) + (-vl) vs (vl+vs) (\sqrt{J^2 + vj^2} - J) + (-vj) vs (vj+vs) (\sqrt{L^2 + vl^2} + L) \right)$

(%i4) /\*  $M_{\{j,j+1\}}^{\{\star\}} c_{\{j+1\}} \omega / c_{\{j\}} = Mm2(J,L,S,vj,vl,vs)$  \*/

$Mm2(J,L,S,vj,vl,vs) := (1/(2 \cdot vj \cdot S \cdot ((J-S)^2 - L^2))) \cdot ((J-S + \sqrt{L^2 + vl^2}) \cdot (vs \cdot (vj+vl) \cdot (\sqrt{J^2 + vj^2} - J) + vj \cdot (vl+vs) \cdot (\sqrt{S^2 + vs^2} + S) - vj \cdot vs \cdot (vj+vs)) + vl \cdot (vj+vs) \cdot (\sqrt{J^2 + vj^2} - J) \cdot (\sqrt{S^2 + vs^2} + S) - vl \cdot vs \cdot (vl+vs) \cdot (\sqrt{J^2 + vj^2} - J) - vj \cdot vl \cdot (vj+vl) \cdot (\sqrt{S^2 + vs^2} + S));$

(%o4)  $Mm2(J,L,S,vj,vl,vs) := \frac{1}{2 vj S \left( (J-S)^2 - L^2 \right)} \left( (J-S + \sqrt{L^2 + vl^2}) \left( vs (vj+vl) (\sqrt{J^2 + vj^2} - J) + vj (vl+vs) (\sqrt{S^2 + vs^2} + S) + (-vj) vs (vj+vs) \right) + vl (vj+vs) \right. \\ \left. (\sqrt{J^2 + vj^2} - J) (\sqrt{S^2 + vs^2} + S) + (-vl) vs (vl+vs) (\sqrt{J^2 + vj^2} - J) + (-vj) vl (vj+vl) (\sqrt{S^2 + vs^2} + S) \right)$

```

(%i5) /* Definition (142) */
/* \gamma_{a}/\omega=A, \gamma_{b}/\omega=B */
/* \tilde{v}_{a}=va, \tilde{v}_{b}=vb, \tilde{v}_{a+b}=vab */
/* K_{a,b}^{+}c_{b}\omega/c_{a}=K(A,B,va,vb,vab) */

K(A,B,va,vb,vab):=(1/(4*va*vab*B*(A+B)))*((sqrt((A+B)^2+vab^2)+A+B)
*(vb+vab)*(sqrt(A^2+va^2)-A)*(sqrt(B^2+vb^2)+B)-vb*(va+vb)*(sqrt(A^2+va^2)-A)
+va*vab*(va+vab))+va*vab*(va+vb)*(sqrt(B^2+vb^2)+B)-va*vab*(vb+vab)
-vab*(va+vab)*(sqrt(A^2+va^2)-A)*(sqrt(B^2+vb^2)+B));

(%o5) K(A,B,va,vb,vab):=

$$\frac{1}{4 va vab B (A+B)} \left( \left( \sqrt{(A+B)^2 + vab^2} + A + B \right) \right.$$


$$\left. \left( (vb+vab) \left( \sqrt{A^2 + va^2} - A \right) \left( \sqrt{B^2 + vb^2} + B \right) - vb (va+vb) \left( \sqrt{A^2 + va^2} - A \right) + va vab (va+vab) \right) + va vab \right.$$


$$\left. (va+vb) \left( \sqrt{B^2 + vb^2} + B \right) + (-va) vb vab (vb+vab) + (-vab) (va+vab) \left( \sqrt{A^2 + va^2} - A \right) \left( \sqrt{B^2 + vb^2} + B \right) \right)$$


(%i6) /* Equality (134) */

ratsimp(Mp1(J,L,S,vj,vl,vs)-Mp2(J,L,S,vj,vl,vs)+Mm1(J,L,S,vj,vl,vs)-Mm2(J,L,S,vj,vl,vs));

(%o6) 0

(%i7) /* Equality (138) (see formula (137)) */

ratsimp(((J+L-sqrt(S^2+vs^2))*vl/((sqrt(L^2+vl^2)-L)*vs))*Mp1(J,L,S,vj,vl,vs)
-((J+S-sqrt(L^2+vl^2))*vs/((sqrt(S^2+vs^2)-S)*vl))*Mp2(J,L,S,vj,vl,vs)
+((J-L-sqrt(S^2+vs^2))*vl/((sqrt(L^2+vl^2)+L)*vs))*Mm1(J,L,S,vj,vl,vs)
-((J-S-sqrt(L^2+vl^2))*vs/((sqrt(S^2+vs^2)+S)*vl))*Mm2(J,L,S,vj,vl,vs)
+(vj+vs)/vl-(vj+vl)/vs+(1/vs-1/vl)*(sqrt(J^2+vj^2)-J));

(%o7) 0

```

```
(%i8) /* Equality (140) (see formula (139)) */
```

```
ratsimp(L·Mp1(J,L,S,vj,vl,vs)+(J+S)·Mp2(J,L,S,vj,vl,vs)
-L·Mm1(J,L,S,vj,vl,vs)+(J-S)·Mm2(J,L,S,vj,vl,vs)-(vl+vs));
```

```
(%o8) 0
```

```
(%i9) /* Equality (143) (see formula (141)) */
```

```
ratsimp(K(A,B,va,vb,vab)-(2/(vb·(sqrt((A+B)^2+vab^2)-A-B)))
·((A+B)·(2·A+B-sqrt(B^2+vb^2))·Mp2(A,B,A+B,va,vb,vab)
+B·(sqrt(B^2+vb^2)-B)·Mm1(A,B,A+B,va,vb,vab))
+(1/(2·va·vb·(sqrt((A+B)^2+vab^2)-A-B)))
·(2·va·vab·(va+vab)-2·va·(vb+vab)·(sqrt((A+B)^2+vab^2)-A-B)-2·vab·(va+vb)·(sqrt(A^2+va^2)-A)
-vb·(va+vab)·(sqrt(A^2+va^2)-A)·(sqrt(B^2+vb^2)-B)/B-va·vb^2·(vb+vab)/B
+va·vb·(va+vb)·(sqrt(B^2+vb^2)-B)/B);
```

```
(%o9) 0
```

```
(%i10) /* Equality (145) (see formula (144)) */
```

```
ratsimp(((sqrt((A+B)^2+vab^2)-A-B)·vb)/((sqrt(B^2+vb^2)+B)·vab))·K(A,B,va,vb,vab)
+(2/vab)·((A+B)·Mp2(A,B,A+B,va,vb,vab)-B·Mm1(A,B,A+B,va,vb,vab))-(1/(2·va·vab·B))
·(vb·(va+vab)·(sqrt(A^2+va^2)-A)+va·(vb+vab)·(sqrt(B^2+vb^2)+B)-va·vb·(va+vb));
```

```
(%o10) 0
```
